# Supplementary material for: Detecting the oldest geodynamo and attendant shielding from the solar wind: Implications for habitability
Source: arXiv:1502.04410 source file (2015-02-16)
Supplement: Supplementary file 1 [file Supplementary_Content.pdf]

**Supplementary Content for “Detecting the oldest geodynamo and attendant shielding from the solar wind: Implications for habitability” by J.A. Tarduno, E.G. Blackman and E.E. Mamajek**

**Reconstructing the Past Sun**

We combine a theoretical stellar evolutionary track for a  $1 M_{\odot}$  star with observational constraints on the time-evolution of various stellar parameters for Sun-like stars to produce a reconstruction of the Sun’s characteristics at geologically and astronomically relevant times (see following table). The solar parameters are listed at the starts of various geological time periods, adopting recent ages from the Geological Society of America (Walker et al., 2013). We adopt the  $1 M_{\odot}$  stellar evolutionary track from Bressan et al. (2012), which employs the recent Caffau et al. (2011) mixture for protosolar chemical composition. We make minor systematic shifts to the luminosity and effective temperature of the evolutionary track at the  $\sim 1\%$  level in order to match the current Sun at an adopted meteoritic age for the solar system (4568 Myr; Bouvier and Wadhwa, 2010; Amelin et al., 2010). We adopt the revised stellar parameters compiled by Mamajek (2012): effective temperature  $T_{\text{eff}} = 5772$  K, luminosity  $L = 3.827 \times 10^{33}$  erg s $^{-1}$ , and radius  $R = 695660$  km. Spectral types were estimated through the new main sequence effective temperature scale of Mamajek and Pecaat (2013) (although in practice spectral types for G-stars are rarely quoted to better than  $\pm 1$  subtype precision). The X-ray luminosity evolution as a function of rotation was calibrated to the data from Wright et al. (2011), but was adjusted to pass through the Sun’s current combination of average X-ray luminosity and rotation period (parameterized via Rossby number; Mamajek and Hillenbrand, 2008). We have included an estimate of the mean emission-measure-averaged coronal temperature  $\log \tilde{T}_X$  as a function of the Sun’s age, based on a custom fit to the data of Telleschi et al. (2005) and the modern Sun (Peres et al., 2000) as a function of mean X-ray luminosity in the ROSAT X-ray bandpass ( $L_X$ ):  $\log \tilde{T}_X \simeq -1.54 + 0.282 \log L_X$  ( $L_X$  in erg s $^{-1}$ ).

We estimate the Sun’s current average solar wind mass loss as follows. Based on  $\sim 15,000$  daily solar wind measurements in the OmniWeb database<sup>1</sup> between 1963 and 2014, we estimate a mean daily solar wind density of  $n = 6.94$  cm $^{-3}$  and mean solar wind velocity of  $V_{SW} = 439$  km s $^{-1}$ . Extrapolating these values over  $4\pi$  steradians, one would estimate the solar wind mass loss rate to be  $1.94 \times 10^{-14} M_{\odot}$  yr $^{-1}$ . Results from the Ulysses mission (Goldstein et al., 1996) show that at high heliographic latitude ( $>20^{\circ}$ ) the solar wind has a product of density and velocity approximately half that at lower latitudes. We take this result into account and multiple our original estimate by  $\sim 2/3$ , leading to a spherically-averaged mean solar mass loss via solar wind of  $\dot{M}_{\odot} = 1.3 \times 10^{-14} M_{\odot}$  yr $^{-1}$ .

Three mass loss rates are listed in the table:  $\dot{M}_W$  is estimated following the observational trends from Wood et al. (2014),  $\dot{M}_S$  is estimated following the simulations of Suzuki et al. (2013), and  $\dot{M}_{CME}$  is the estimated mass loss due solely to coronal mass ejections from flares (Drake et al.,

---

<sup>1</sup>Goddard Space Flight Center Space Physics Data Facility: <http://omniweb.gsfc.nasa.gov/>.

2013). Magnetopause radii are estimated following Tarduno et al. (2010), assuming Earth magnetic field strengths equal to the current value ( $R_{S,1}$ ) and half ( $R_{S,1/2}$ ); these field strengths are similar to bounds for the Archean discussed by Tarduno et al. (2010). Interplanetary magnetic field pressure was assumed to be negligible at all periods compared to the dynamical ram pressure of the wind.

Several of the stellar parameters for the Sun and Sun-like stars (mostly related to magnetic activity) are observationally well correlated with rotation period (e.g. Mamajek and Hillenbrand, 2008), so we made a careful reassessment of the Sun’s likely rotational evolution through study of Sun-like main sequence stars of different ages. Based upon a literature review of measured rotation rates of  $\sim 1 M_{\odot}$  ( $\pm 10\%$ ) stars in ten young star clusters<sup>2</sup> and older field stars<sup>3</sup> we derive a revised version of the Skumanich law (Skumanich, 1972):  $P_{rot} = 25.5(t/t_{\odot})^{0.526 \pm 0.022}$  day, where  $t$  is stellar age,  $t_{\odot}$  is the Sun’s age (4568 Myr), and the relation is empirically constrained between  $\sim 0.1$ -7 Gyr. A fit of Sun-like stars in young clusters and (older) field stars *omitting* the Sun, yields a nearly identical relation, *predicting* the modern Sun’s rotation period to be 25.4 day. We surmise that the Sun is a normal rotator (within  $\pm 1$  day) for its mass and age.

Has mass loss via the solar wind had an impact on the Sun’s luminosity evolution since reaching the main sequence? An enhanced early solar wind has been proposed to be a potential solution to the Faint Young Sun paradox (e.g. Sackmann and Boothroyd, 2003). We have surveyed the recent literature for published mass loss estimates and trends for Sun-like stars, as a function of age and/or X-ray luminosity, as well as theoretical predictions (e.g. Holzwarth and Jardine, 2007; Cranmer and Saar, 2011; Drake et al., 2013; Suzuki et al., 2013; Wood et al., 2014). Thus far, these recent studies are consistent with a total solar main sequence mass loss in the range  $\sim 0.01$ -0.4%. In the same period, the Sun has lost  $\sim 0.03\%$  of its mass due to radiative losses through converting mass to energy (Sackmann and Boothroyd, 2003). The Bressan et al. (2012) stellar evolutionary tracks are consistent with having zero-age main sequence luminosities of  $L_{ZAMS} \simeq 0.70 (M/M_{\odot})^{4.535} L_{\odot}$  for solar composition stars within 10% of a solar mass. After 4.6 Gyr, the total predicted solar mass loss due to solar wind and radiative losses is in the range  $\sim 0.04$ -0.4%, so the Sun could have plausibly been negligibly more luminous ( $\sim 0.2$ -1.8%) early in its main sequence phase. Hence, current observational and theoretical constraints on the mass loss history of the Sun seem inconsistent with enhanced early stellar winds providing a parsimonious solution to the Faint Young Sun paradox (e.g. Sackmann and Boothroyd, 2003).

---

<sup>2</sup>In age order: Pleiades, M50, M35, M34, M11, Coma Ber, M37, Praesepe, Hyades, and NGC 6811.

<sup>3</sup>In age order: 18 Sco, Sun,  $\alpha$  Cen A & B (mean), 16 Cyg B.

**Table 1:** Solar Parameters: Zero-Age Main Sequence to Present

| $\tau$<br>Gyr | Age<br>Gyr | $T_{\text{eff}}$<br>K | Spec.<br>Type | Lum.<br>$L/L_{\odot}$ | Rad.<br>$R/R_{\odot}$ | $\log R_X$<br>dex | $\log L_X$<br>$\text{ergs}^{-1}$ | $\log \tilde{\Gamma}_X$<br>K | $\dot{M}_W$<br>$M_{\odot} \text{yr}^{-1}$ | $\dot{M}_S$<br>$M_{\odot} \text{yr}^{-1}$ | $\dot{M}_{CME}$<br>$M_{\odot} \text{yr}^{-1}$ | $R_{S,1}$<br>$R_{Earth}$ | $R_{S,1/2}$<br>$R_{Earth}$ | Name of Starting Geological Period<br>... |
|---------------|------------|-----------------------|---------------|-----------------------|-----------------------|-------------------|----------------------------------|------------------------------|-------------------------------------------|-------------------------------------------|-----------------------------------------------|--------------------------|----------------------------|-------------------------------------------|
| 4.525         | 0.045      | 5630.                 | G5.4V         | 0.686                 | 0.871                 | -3.33             | 30.1                             | 6.96                         | -12.6                                     | -11.5                                     | -10.1                                         | 4.7                      | 3.7                        | Zero-Age Main Sequence (ZAMS)             |
| 4.450         | 0.120      | 5645.                 | G5.2V         | 0.707                 | 0.879                 | -3.92             | 29.5                             | 6.79                         | -13.4                                     | -11.9                                     | -10.9                                         | 5.5                      | 4.4                        | Pleiades Cluster Age                      |
| 4.000         | 0.570      | 5660.                 | G5.0V         | 0.735                 | 0.891                 | -4.85             | 28.6                             | 6.54                         | -12.0                                     | -12.7                                     | -12.3                                         | 7.0                      | 5.6                        | Archaen Eon/Eoarchean Era                 |
| 3.920         | 0.650      | 5662.                 | G4.9V         | 0.739                 | 0.893                 | -4.93             | 28.5                             | 6.51                         | -12.1                                     | -12.8                                     | -12.4                                         | 7.2                      | 5.7                        | Hyaades Cluster Age                       |
| 3.600         | 0.970      | 5672.                 | G4.4V         | 0.756                 | 0.900                 | -5.18             | 28.3                             | 6.45                         | -12.4                                     | -13.0                                     | -12.7                                         | 7.7                      | 6.1                        | Paleoarchean Era                          |
| 3.450         | 1.120      | 5676.                 | G4.2V         | 0.764                 | 0.904                 | -5.27             | 28.2                             | 6.42                         | -12.5                                     | -13.0                                     | -12.9                                         | 7.8                      | 6.2                        | Barberton Greenstone Belt dacite          |
| 3.200         | 1.370      | 5684.                 | G3.9V         | 0.777                 | 0.909                 | -5.40             | 28.1                             | 6.39                         | -12.7                                     | -13.1                                     | -13.1                                         | 8.1                      | 6.4                        | Mesoarchean Era                           |
| 2.800         | 1.770      | 5696.                 | G3.6V         | 0.800                 | 0.918                 | -5.56             | 27.9                             | 6.35                         | -12.9                                     | -13.2                                     | -13.4                                         | 8.4                      | 6.7                        | Neoarchean Era                            |
| 2.500         | 2.070      | 5705.                 | G3.4V         | 0.818                 | 0.926                 | -5.67             | 27.8                             | 6.32                         | -13.0                                     | -13.3                                     | -13.6                                         | 8.6                      | 6.8                        | Proterozoic Eon                           |
| 2.300         | 2.270      | 5710.                 | G3.2V         | 0.830                 | 0.931                 | -5.73             | 27.8                             | 6.30                         | -13.1                                     | -13.4                                     | -13.7                                         | 8.8                      | 6.9                        | Rhyacian Period                           |
| 2.050         | 2.520      | 5718.                 | G3.1V         | 0.846                 | 0.937                 | -5.81             | 27.7                             | 6.28                         | -13.2                                     | -13.4                                     | -13.8                                         | 8.9                      | 7.1                        | Orosirian Period                          |
| 1.800         | 2.770      | 5725.                 | G2.9V         | 0.862                 | 0.944                 | -5.87             | 27.6                             | 6.27                         | -13.3                                     | -13.5                                     | -13.9                                         | 9.0                      | 7.2                        | Strathertian Period                       |
| 1.600         | 2.970      | 5731.                 | G2.8V         | 0.876                 | 0.949                 | -5.92             | 27.6                             | 6.25                         | -13.3                                     | -13.5                                     | -14.0                                         | 9.1                      | 7.2                        | Mesoproterozoic Era                       |
| 1.400         | 3.170      | 5736.                 | G2.7V         | 0.890                 | 0.955                 | -5.97             | 27.6                             | 6.24                         | -13.4                                     | -13.5                                     | -14.1                                         | 9.2                      | 7.3                        | Ectasian Period                           |
| 1.200         | 3.370      | 5742.                 | G2.6V         | 0.904                 | 0.961                 | -6.01             | 27.5                             | 6.23                         | -13.4                                     | -13.6                                     | -14.2                                         | 9.3                      | 7.4                        | Stenian Period                            |
| 1.000         | 3.570      | 5747.                 | G2.5V         | 0.919                 | 0.967                 | -6.06             | 27.5                             | 6.22                         | -13.5                                     | -13.6                                     | -14.2                                         | 9.4                      | 7.5                        | Tonian Period                             |
| 0.850         | 3.720      | 5751.                 | G2.4V         | 0.930                 | 0.971                 | -6.08             | 27.5                             | 6.22                         | -13.5                                     | -13.6                                     | -14.3                                         | 9.4                      | 7.5                        | Cryogenian Period                         |
| 0.635         | 3.935      | 5757.                 | G2.3V         | 0.947                 | 0.978                 | -6.13             | 27.4                             | 6.21                         | -13.6                                     | -13.6                                     | -14.4                                         | 9.5                      | 7.6                        | Ediacaran Period                          |
| 0.541         | 4.029      | 5759.                 | G2.2V         | 0.954                 | 0.981                 | -6.15             | 27.4                             | 6.20                         | -13.6                                     | -13.6                                     | -14.4                                         | 9.6                      | 7.6                        | Cambrian Period                           |
| 0.485         | 4.085      | 5760.                 | G2.2V         | 0.959                 | 0.983                 | -6.15             | 27.4                             | 6.20                         | -13.6                                     | -13.7                                     | -14.4                                         | 9.6                      | 7.6                        | Ordovician Period                         |
| 0.444         | 4.126      | 5762.                 | G2.2V         | 0.962                 | 0.985                 | -6.17             | 27.4                             | 6.20                         | -13.6                                     | -13.7                                     | -14.4                                         | 9.6                      | 7.6                        | Silurian Period                           |
| 0.419         | 4.151      | 5762.                 | G2.2V         | 0.964                 | 0.985                 | -6.17             | 27.4                             | 6.20                         | -13.6                                     | -13.7                                     | -14.4                                         | 9.6                      | 7.6                        | Devonian Period                           |
| 0.359         | 4.211      | 5764.                 | G2.2V         | 0.969                 | 0.987                 | -6.18             | 27.4                             | 6.20                         | -13.6                                     | -13.7                                     | -14.5                                         | 9.6                      | 7.6                        | Carboniferous Period                      |
| 0.299         | 4.271      | 5765.                 | G2.1V         | 0.974                 | 0.990                 | -6.19             | 27.4                             | 6.19                         | -13.7                                     | -13.7                                     | -14.5                                         | 9.7                      | 7.7                        | Permian Period                            |
| 0.252         | 4.318      | 5766.                 | G2.1V         | 0.978                 | 0.991                 | -6.20             | 27.4                             | 6.19                         | -13.7                                     | -13.7                                     | -14.5                                         | 9.7                      | 7.7                        | Triassic Period                           |
| 0.201         | 4.369      | 5767.                 | G2.1V         | 0.983                 | 0.993                 | -6.21             | 27.4                             | 6.19                         | -13.7                                     | -13.7                                     | -14.5                                         | 9.7                      | 7.7                        | Jurassic Period                           |
| 0.145         | 4.425      | 5769.                 | G2.1V         | 0.988                 | 0.995                 | -6.22             | 27.4                             | 6.19                         | -13.7                                     | -13.7                                     | -14.5                                         | 9.7                      | 7.7                        | Cretaceous Period                         |
| 0.066         | 4.504      | 5771.                 | G2.0V         | 0.994                 | 0.998                 | -6.23             | 27.3                             | 6.18                         | -13.7                                     | -13.7                                     | -14.5                                         | 9.7                      | 7.7                        | Paleogene Period                          |
| 0.023         | 4.547      | 5771.                 | G2.0V         | 0.998                 | 0.999                 | -6.24             | 27.3                             | 6.18                         | -13.7                                     | -13.7                                     | -14.6                                         | 9.7                      | 7.7                        | Neogene Period                            |
| 0.003         | 4.567      | 5772.                 | G2.0V         | 1.000                 | 1.000                 | -6.24             | 27.3                             | 6.18                         | -13.7                                     | -13.7                                     | -14.6                                         | 9.7                      | 7.7                        | Quaternary Period                         |

- Amelin, Y., Kaltenbach, A., Iizuka, T., Stirling, C.H., Ireland, T.R., Petaev, M., Jacobsen, S.B., 2010. U-Pb chronology of the Solar System's oldest solids with variable  $^{238}\text{U}/^{235}\text{U}$ . *Earth and Planetary Science Letters* 300, 343–350. doi:10.1016/j.epsl.2010.10.015.
- Bouvier, A., Wadhwa, M., 2010. The age of the Solar System redefined by the oldest Pb-Pb age of a meteoritic inclusion. *Nature Geoscience* 3, 637–641. doi:10.1038/ngeo941.
- Bressan, A., Marigo, P., Girardi, L., Salasnich, B., Dal Cero, C., Rubele, S., Nanni, A., 2012. PAR-SEC: stellar tracks and isochrones with the PAdova and TRieste Stellar Evolution Code. *Monthly Notices of the Royal Astronomical Society* 427, 127–145. doi:10.1111/j.1365-2966.2012.21948.x.
- Caffau, E., Ludwig, H.G., Steffen, M., Freytag, B., Bonifacio, P., 2011. Solar Chemical Abundances Determined with a CO5BOLD 3D Model Atmosphere. *Solar Physics* 268, 255–269. doi:10.1007/s11207-010-9541-4.
- Cranmer, S.R., Saar, S.H., 2011. Testing a Predictive Theoretical Model for the Mass Loss Rates of Cool Stars. *The Astrophysical Journal* 741, 54. doi:10.1088/0004-637X/741/1/54.
- Drake, J.J., Cohen, O., Yashiro, S., Gopalswamy, N., 2013. Implications of Mass and Energy Loss due to Coronal Mass Ejections on Magnetically Active Stars. *The Astrophysical Journal* 764, 170. doi:10.1088/0004-637X/764/2/170.
- Goldstein, B.E., Neugebauer, M., Phillips, J.L., Bame, S., Gosling, J.T., McComas, D., Wang, Y.M., Sheeley, N.R., Suess, S.T., 1996. ULYSSES plasma parameters: latitudinal, radial, and temporal variations. *Astronomy and Astrophysics* 316, 296–303.
- Holzwarth, V., Jardine, M., 2007. Theoretical mass loss rates of cool main-sequence stars. *Astronomy and Astrophysics* 463, 11–21. doi:10.1051/0004-6361:20066486.
- Mamajek, E.E., 2012. On the Age and Binarity of Fomalhaut. *The Astrophysical Journal Letters* 754, L20. doi:10.1088/2041-8205/754/2/L20.
- Mamajek, E.E., Hillenbrand, L.A., 2008. Improved Age Estimation for Solar-Type Dwarfs Using Activity-Rotation Diagnostics. *The Astrophysical Journal* 687, 1264–1293. doi:10.1086/591785.
- Mamajek, E.E., Pecaat, M.J., 2013. Intrinsic colors, temperatures, and bolometric corrections of pre-main sequence stars. *The Astrophysical Journal Supplement Series* 208, 9.
- Peres, G., Orlando, S., Reale, F., Rosner, R., Hudson, H., 2000. The sun as an x-ray star. ii. using the yokkoh/soft x-ray telescope-derived solar emission measure versus temperature to interpret stellar x-ray observations. *The Astrophysical Journal* 528, 537–551.
- Sackmann, I.J., Boothroyd, A.I., 2003. Our Sun. V. A Bright Young Sun Consistent with Helioseismology and Warm Temperatures on Ancient Earth and Mars. *The Astrophysical Journal* 583, 1024–1039. doi:10.1086/345408.

- Skumanich, A., 1972. Time Scales for CA II Emission Decay, Rotational Braking, and Lithium Depletion. *The Astrophysical Journal* 171, 565. doi:10.1086/151310.
- Suzuki, T.K., Imada, S., Kataoka, R., Kato, Y., Matsumoto, T., Miyahara, H., Tsuneta, S., 2013. Saturation of Stellar Winds from Young Suns. *Publications of the Astronomical Society of Japan* 65, 98. doi:10.1093/pasj/65.5.98.
- Tarduno, J.A., Cottrell, R.D., Watkeys, M.K., Hofmann, A., Doubrovine, P.V., Mamajek, E.E., Liu, D., Sibeck, D.G., Neukirch, L.P., Usui, Y., 2010. Geodynamo, solar wind, and magnetopause 3.4 to 3.45 billion years ago. *Science* 327, 1238–1240. doi:10.1126/science.1183445.
- Telleschi, A., Güdel, M., Briggs, K., Audard, M., Ness, J.U., , Skinner, S.L., 2005. Coronal evolution of the sun in time: High-resolution x-ray spectroscopy of solar analogs with different ages. *The Astrophysical Journal* 622, 653–679.
- Walker, J.D., Geissman, J.W., Bowring, S.A., Babcock, L.E., 2013. The Geological Society of America Geologic Time Scale. *Geological Society of America Bulletin* 125, 259–272. doi:10.1130/B30712.1.
- Wood, B.E., Müller, H.R., Redfield, S., Edelman, E., 2014. Evidence for a Weak Wind from the Young Sun. *The Astrophysical Journal Letters* 781, L33. doi:10.1088/2041-8205/781/2/L33.
- Wright, N.J., Drake, J.J., Mamajek, E.E., Henry, G.W., 2011. The stellar-activity-rotation relationship and the evolution of stellar dynamos. *The Astrophysical Journal* 743.
